# Supplementary material for: Spike-Triggered Descent
Source: arXiv:2005.05572 source file (2020-05-12)
Supplement: Supplementary file 2 [file appendix-ND1Order.tex]

\documentclass[../main.tex]{subfiles}
\begin{document}

\begin{equation} \label{eq:GCSRMp}
\begin{split}
\tilde{\Theta} = & K_0 + \sum_{n=1}^N \idotsint_n K(\tau_{1 \rightarrow n}; \beta_{i,l}) \prod_{i = 1}^n x(t_l^O - \tau_i) d\tau_i + \sum \eta(t_l^O - t_k^O; \mu_k)
\\ \\= &(K_0 + \Delta K_0)+ \sum_{n=1}^N \idotsint_n \Big[K(\tau_{1 \rightarrow n}; \beta_{i,l} + \Delta \beta_{i,l})\Big] 
\prod_{j = 1}^n
\Big[x(t_l^O + \Delta t_l^O - \tau_j)
\Big] 
d\tau_j
\\ &
+ \sum \eta(t_l^O + \Delta t_l^O - t_k^O - \Delta t_k^O; \mu_k + \Delta \mu_k)
\\ \\ = & (K_0 + \Delta K_0)
\\ & + \sum_{n=1}^N  \idotsint_n
\Big[ K(\tau_{1 \rightarrow n}; \beta_{i,l}) + \sum B_i(\tau_{1 \rightarrow n}) \Delta \beta_{i,l}\Big]
\prod_{j = 1}^n
\Big[ x(t_l^O - \tau_j) + \frac{\partial x}{\partial t} \Big|_{t_l^O - \tau_j} \Delta t_l^O 
\Big] 
d\tau_j
\\ &
+ \sum \Big[ \eta(t_l^O - t_k^O; \mu_k)
+ \frac{\partial \eta}{\partial t} \Big|_{t_l^O - t_k^O} (\Delta t_l^O - \Delta t_k^O) 
+ \frac{\partial \eta}{\partial \mu} \Big|_{t_l^O - t_k^O} (\Delta \mu_k) \Big]
\end{split}
\end{equation}

\begin{equation} \label{eq:GCSRMc}
\begin{split}
0 = \Delta K_0 &
+ 
\sum_{n=1}^N  \idotsint_n
\Big[\sum B_i(\tau_{1 \rightarrow n}) \Delta \beta_{i,l}\Big]
\Big[
\prod_{j = 1}^n
x(t_l^O - \tau_j)
d\tau_j
\Big]
\\ & + 
\sum_{n=1}^N  \idotsint_n
K(\tau_{1 \rightarrow n}; \beta_{i,l})
\Big[
\sum_{m=1}^n
\Big[ 
\prod_{j \ne m}^n
x(t_l^O - \tau_j)
\Big]
\frac{\partial x}{\partial t} \Big|_{t_l^O - \tau_m} \Delta t_l^O
\Big]
\prod_{j = 1}^n
d\tau_j
\\ &
+ \sum \Big[ \frac{\partial \eta}{\partial t} \Big|_{t_l^O - t_k^O} (\Delta t_l^O - \Delta t_k^O) 
+ \frac{\partial \eta}{\partial \mu} \Big|_{t_l^O - t_k^O} (\Delta \mu_k)\Big]
\end{split}
\end{equation}

\begin{equation} \label{eq:GCSRMdt}
\resizebox{.9\hsize}{!}{$
\Delta t_l^O = 
\frac{
\sum \frac{\partial \eta}{\partial t} \big|_{t_l^O - t_k^O}  \Delta t_k^O
-
\sum \frac{\partial \eta}{\partial \mu} \big|_{t_l^O - t_k^O} \Delta \mu_k
-
\Delta K_0
- 
\sum_{n=1}^N  \idotsint_n
(\sum B_i(\tau_{1 \rightarrow n}) \Delta \beta_{i,l})
\prod_{j = 1}^n
x(t_l^O - \tau_j)
d\tau_j
}
{
\sum_{n=1}^N  \idotsint_n
K(\tau_{1 \rightarrow n}; \beta_{i,l})
\Big[
\sum_{m=1}^n
\Big[ 
\prod_{j \ne m}^n
x(t_l^O - \tau_j)
\Big]
\frac{\partial x}{\partial t} \big|_{t_l^O - \tau_m} 
\Big]
\prod_{j = 1}^n
d\tau_j
+ \sum \frac{\partial \eta}{\partial t} \big|_{t_l^O - t_k^O}
}
$}
\end{equation}

\end{document}
